# Supplementary material for: Nonequilibrium many-body dynamics in supersymmetric quenching
Source: arXiv:2203.03130 source file (2022-07-21)
Supplement: Supplementary file 1 [file appendix.tex]

\section{Analytical Expression for Supersymmetric Wavefunction of the infinite box} \label{app:infinite_box}
Throughout this paper we have defined our starting potential as an infinite box the is centered around the origin. The wavefunctions for this potential are written as
\begin{equation}
  \psi^{(1)}_n(x)=\begin{cases}
    \sqrt{\frac{2}{L}}\text{sin}(\frac{n x\pi}{L}), & \; n = even;,\\
    \sqrt{\frac{2}{L}}\text{cos}\left(\frac{n x\pi}{L}\right), & \; n = odd;
  \end{cases}
\end{equation}
with the ground state being $\psi^{(1)}_0 = \sqrt{\frac{2}{L}}\cos{\frac{x\pi}{L}}$. Using Eq.~\eqref{eq:superpot} the superpotential is calculated using the annihilation operator on the ground state and we find 
\begin{equation}
        W^{(2)}(x)  = \frac{\pi}{\sqrt{2}L}\frac{\text{sin}\left(\frac{x\pi}{L}\right)}{\text{cos}\left(\frac{x\pi}{L}\right)}= \frac{\pi}{\sqrt{2}L}\text{tan}\left(\frac{x\pi}{L}\right)\;.
\end{equation}
Once the superpotential is found the analytical wavefunctions of the partner potential $V^{(2)}$ can be found by using the anihilation operator on each wavefunction. The first 4 eigenstates of $V^{(2)}$ are 
\begin{align}
    \psi^{(2)}_1(x)&\propto \frac{\pi}{L^{3/2}}\left(\frac{\text{sin}(\frac{x\pi}{L})\text{sin}(\frac{2x\pi}{L})}{\text{cos}(\frac{x\pi}{L})} + 2\text{cos}(\frac{2x\pi}{L})\right)\nonumber\\
    \psi^{(2)}_2(x)&\propto\frac{\pi}{L^{3/2}}\left( \frac{\text{sin}(\frac{x\pi}{L})\text{cos}(\frac{3x\pi}{L})}{\text{cos}(\frac{x\pi}{L})}-3\text{sin}(\frac{3x\pi}{L})\right)\nonumber\\
    \psi^{(2)}_3(x)&\propto \frac{\pi}{L^{3/2}}\left(\frac{\text{sin}(\frac{x\pi}{L})\text{sin}(\frac{4x\pi}{L})}{\text{cos}(\frac{x\pi}{L})}+  4\text{cos}(\frac{4x\pi}{L}) \right)\nonumber\\
    \psi^{(2)}_4(x)&\propto\frac{\pi}{L^{3/2}}\left( \frac{\text{sin}(\frac{x\pi}{L})\text{cos}(\frac{5x\pi}{L})}{\text{cos}(\frac{x\pi}{L})}-5\text{sin}(\frac{5x\pi}{L})\right)\nonumber\\
\end{align}
and more generally 
\begin{equation}
  \psi^{(2)}_{m-1}(x)\propto\begin{cases}
    \frac{\pi}{L^{3/2}}(m\text{cos}(\frac{mx\pi}{L}) + \frac{\text{sin}(\frac{x\pi}{L})\text{sin}(\frac{mx\pi}{L})}{\text{cos}(\frac{x\pi}{L})}), m = even\\
    \frac{\pi}{L^{3/2}}( \frac{\text{sin}(\frac{x\pi}{L})\text{cos}(\frac{mx\pi}{L})}{\text{cos}(\frac{x\pi}{L})}-m\text{sin}(\frac{mx\pi}{L})), m = odd\\
  \end{cases}\nonumber
\end{equation}
where the transformed wavefunction are to be normalized using the difference in energy between the ground state of the starting potential with the energy of the state where the annihilation operator is applied as mentioned in Eq.~\eqref{eq:WFIntertwine}. If this process is repeated on the new ground we find that the superpotential can be written in a general form 
In general, and for all subsequent partner potentials 
\begin{equation}
    W^{(\alpha)} = (\alpha - 1)\frac{\pi}{\sqrt{2}L}\text{tan}\left(\frac{x\pi}{L}\right)\;,
\end{equation}
where $\alpha = 2,3,4, ... $ is the target potential. Consequently this makes the supersymmetric operators
\begin{equation}
    A^{(\alpha)} = \frac{1}{\sqrt{2}}\frac{\partial}{\partial x} + W^{(\alpha)}(x);.
\end{equation}
It is worth noting that a more general description of wavefunctions of the infinite box wavefunctions with a shifted centered can be described by the Chebyshev polynomials of the first and second kind which can also be used to find the values as described above, with the superpotential changing from a tan function to a cotangent function \cite{infinite_well_SUSY:2018}.

\section{Wavefunction Revival for Supersymmetric infinite box}\label{app:Revival}
%A Taylor series expansion of the energy with respect to the principle quantum number shows different periods and the second derivative is the wavefunction revival period. This provides us with a universal time scale to describe the dynamics of the system. Starting with the weighted probabilities of the overlaps, we can expand the energy of the most predominant excitation around $\Tilde{n}$ using a Taylor's expansion with respect to the quantum principle number. From the following expansion of the energy
%\begin{equation}
 %   E_n \approx E_{\Tilde{n}} + E^{'}_{\Tilde{n}}\left(n - \Tilde{n}\right) + \frac{1}{2}E^{''}_{\Tilde{n}}\left(n - \Tilde{n}\right)^2 +\frac{1}{6}E^{'''}_{\Tilde{n}}\left(n - \Tilde{n}\right)^3+...
%\end{equation}
%we can obtain time scales which define various periods of the system such as the classical period ($T_{cl}$), the revival time ($t_{rev}$)and the superrevival time ($t_{sup}$),
%\begin{equation}
%    T_{cl} = \frac{2\pi}{|E^{'}_{\Tilde{n}}|}\quad t_{rev} = \frac{4\pi}{|E^{''}_{\Tilde{n}}|}\quad t_{sup} =\frac{12\pi}{|E^{'''}_{\Tilde{n}}|}.
%\end{equation}
\cite{Bluhm:WF_Revival:1996}For the infinite box of length $L$ centered around the origin the energy levels in terms of a quantum principle number is
\begin{equation}
    E(n) = \frac{n^2 \pi^2 \hbar^2}{2mL^2}.
\end{equation}
Except for the ground state these energies are the same for the infinite boxes partner potentials, where the quantum number is $n+1$ instead of just $n$. For both the infinite box and its supersymmetric partners we can take the second derivative of this we obtain
\begin{equation}
    \frac{\partial^2E}{\partial n^2} = \frac{4  \pi^2 \hbar^2}{m L^2}
\end{equation}
in which we define the revival time
\begin{equation}
    t_r = 2\pi \hbar \left(\frac{1}{2}\frac{\partial^2E}{\partial n^2}\right)^{-1}.
\end{equation}
Reducing the equation where $\hbar = m = 1$ applying this to our equation for the revival time we obtain
\begin{equation}
    t_{rev} = \frac{4L^2}{\pi}
\end{equation}
for an infinite box of length $L$. These revival times are normalized to the ground state of the subsequent quenching potential. 
%\subsection{Fractional revivals (why $t_r/4$)}

%\cite{fractional_rev:2005} \cc{we don't need this section anymore.} This is a derivation that looks into Phase difference equations. They start with the revival time and state this must satisfy
%\begin{equation}
 %   \exp[-i2\pi(t/t_r)n^2] = \exp[-i\beta]
%\end{equation}
%For a phase induced by the transition between two energy levels in of energy $E_n$ and $E_m$ within a set of populated energy levels the time in terms of the revival time of the potential is 
%\begin{equation}
 %   t_{n,m} = \frac{t_r}{n^2-m^2}.
%\end{equation}
%this eludes to the first revival of the wavefunction being the least common multiple of the times given for all possible pairs. And the revival time can be written as 
%\begin{equation}
 %   t = \frac{t_r}{\text{gcd}(n^2-m^2)}
%\end{equation}
%I imagine this is an autocorrelation function of an excitation in the same potential however this ties in well with our SUSY quenches. This is then generalized into the idea of ladder excitations where they generalize a base level ($b$) and an integer number of energy spacings (principle numbers i'm assuming) ($dj$), which boils down to the difference in energy levels

%%%%%%%%%%%%%%%%%%%

\section{Average Work and Irreversible Work}\label{app:work}

As mentioned above the irreversible work, average work and free energy reduces to simply equations when written in terms of supersymmetric nomenclature. Plotting this as a function of particle number in Fig.~\ref{fig:work_irrwork} we can see that the irreversible and average work increases 

\begin{figure}[tb]
    \centering
    \includegraphics[width =\linewidth]{Work_irrwork.png}
    \caption{Average work (solid lines) and irreversible work (dashed lines) for supersymmetric quenches from an infinite box to potentials $V^{(2)}$ (black) $V^{(3)}$ (blue) and $V^{(4)}$ (red)}
    \label{fig:work_irrwork}
\end{figure}
%\subsection{Second Example: $W(x) =x^3$}

%So far we have chosen a potential in which the wavefunction, energy levels and as a result the superpotential is analytically known. This allows us to provide a solid case example in a way that allows us to explore many different properties for our supersymmetric treatment of quenching dynamics at $T = 0$. It's important to note that the derivations laid out in this section are not limited to to a box potential. For a pair of potentials with one non-degenerate state, one can define a superpotential (for example $W(x) = x^3$) and test if the potentials produced by this will return a normalizable ground state wavefunction. If this can be accomplished similar quenches can be implemented. The problem then lies in the dependence of the principle quantum number in the classical period and revival time of a wavefunction. Using $W(x) = x^3$ and quenching for different particle numbers, one can obtain revivals in a system however one can observe qualitatively that the number of particles that are used to quench the system affect the revivals, which is an indication that the revival time is state dependent in some way. 

%\begin{figure}[tbh]
 %   \centering
  %  \includegraphics[width =\linewidth]{LE_TWO_POT.png}
   % \caption{Comparison of two quenches. a) Our main example of an infinite box quenching to its first partner potential. b) A quench between two potentials sharing the same superpotential $W(x) = x^3$.}
   % \label{fig:LE_TWO_POT}

%\end{figure}
